# Supplementary material for: Local transfer learning Gaussian process modeling, with applications to surrogate modeling of expensive computer simulators
Source: arXiv:2410.12690 source file (2025-07-11)
Supplement: Supplementary file 1 [file ex_supplement.pdf]

# SUPPLEMENTARY MATERIALS: Local transfer learning Gaussian process modeling, with applications to surrogate modeling of expensive computer simulators

Xinming Wang*, Simon Mak†, John Miller‡, and Jianguo Wu§

**SM1. Gibbs sampling with potentially shared design points.** In the main text, we presumed for notational brevity that no design points are shared between the source and target systems for the multi-source LOL-GP set-up. Our Gibbs sampler extends naturally to the setting with potentially shared design points between source and target. The only modification needed is to replace $\mathbf{\Theta}$ with the new latent parameter set $\mathbf{\Theta}' = \{\{f_l(\mathcal{X}_T \setminus \mathcal{X}_l)\}_{l=1}^L, \{\omega_l(\mathcal{X}_T)\}_{l=1}^L\}$. The sole difference between $\mathbf{\Theta}$ and $\mathbf{\Theta}'$ is the latent function values for $f_l$, where the latter omits the target design points in $\mathcal{X}_T$ that are in the source design $\mathcal{X}_l$. With the new latent parameter set $\mathbf{\Theta}'$, we can employ the same Gibbs sampler from Algorithm 3.1 on each parameter $\theta \in \mathbf{\Theta}'$ to sample from the posterior distribution $[\mathbf{\Theta}'|\text{data}]$. The posterior predictive sampler for $[f_T(\mathbf{x}_{\text{new}})|\text{data}]$ remains unchanged.

Similarly, for the multi-fidelity LOL-GP, we presumed for notational brevity in the main text that no design points are shared between any two fidelity levels. Our Gibbs sampler again extends naturally to the setting where there are potentially shared design points. The only modification needed is to replace $\mathbf{\Theta}_l$ with the new latent parameter set $\mathbf{\Theta}_l' = \{\boldsymbol{f}_l(\mathcal{X}_{(l+1)} \setminus \mathcal{X}_l), \boldsymbol{\omega}_l(\mathcal{X}_{(l+1)})\}$. The sole difference between $\mathbf{\Theta}$ and $\mathbf{\Theta}'$ is again the latent function values for $f_l$, where the latter omits design points in $\mathcal{X}_{(l+1)}$ that are in $\mathcal{X}_l$. With the new latent parameter set $\mathbf{\Theta}_l'$, the same Gibbs sampler from Algorithm 3.2 can be employed for each parameter $\theta \in \mathbf{\Theta}'$ to sample from the posterior distribution $[\{\mathbf{\Theta}_1', \cdots, \mathbf{\Theta}_L'\}|\text{data}]$. The posterior predictive sampler on $[f_T(\mathbf{x}_{\text{new}})|\text{data}]$ again remains unchanged.

**SM2. Full conditional distribution of latent weights in the multi-source LOL-GP.** Given the data $= \{\boldsymbol{f}_1, \cdots, \boldsymbol{f}_L, \boldsymbol{f}_T\}$ and the latent parameters $\mathbf{\Theta}_- = \mathbf{\Theta} \setminus \omega_l(\boldsymbol{x}_i)$, the conditional distribution on $\omega_l(\boldsymbol{x}_i)$ can be expressed as:

$$[\omega_l(\boldsymbol{x}_i)|\text{data}, \mathbf{\Theta}_-] \propto [f_T(\boldsymbol{x}_i)|\omega_l(\boldsymbol{x}_i), \text{data}_-, \mathbf{\Theta}_-][\omega_l(\boldsymbol{x}_i)|\text{data}_-, \mathbf{\Theta}_-], \tag{SM2.1}$$

where $\text{data}_- = \text{data} \setminus f_T(\boldsymbol{x}_i)$. Recall the formulation of the multi-source LOL-GP:

$$\begin{aligned} f_T(\boldsymbol{x}) &= \sum_{l=1}^L \rho_l(\boldsymbol{x}) f_l(\boldsymbol{x}) + \delta(\boldsymbol{x}) \\ &= \text{ReLU}\{\omega_l(\boldsymbol{x})\} f_l(x) + \sum_{l' \neq l} \rho_{l'}(\boldsymbol{x}) f_{l'}(\boldsymbol{x}) + \delta(\boldsymbol{x}). \end{aligned}$$

*Department of Industrial Engineering and Management, Peking University
†Department of Statistical Science, Duke University (sm769@duke.edu)
‡Department of Statistical Science, Duke University
§Department of Industrial Engineering and Management, Peking University (j.wu@pku.edu.cn)
**Funding:** The authors gratefully acknowledge support from NSF CSSI 2004571, NSF DMS 2210729, NSF DMS 2316012 and DE-SC0024477.

The joint distribution of $f_T(\mathcal{X}_T)$ follows:

$$\begin{aligned}&f_T(\mathcal{X}_T)|\{\text{data} \setminus f_T(\mathcal{X}_T)\}, \mathbf{\Theta}_-\\&\sim \mathcal{N}\left\{\text{ReLU}\{\omega_l(\mathcal{X}_T)\} \odot f_l(\mathcal{X}_T) + \sum_{l'\neq l} \rho_{l'}(\mathcal{X}_T) \odot f_{l'}(\mathcal{X}_T),\ \boldsymbol{K}_\delta(\mathcal{X}_T, \mathcal{X}_T)\right\}.\end{aligned}$$

Therefore, the first term in (SM2.1) follows the marginal distribution:

$$\begin{aligned}&f_T(\boldsymbol{x}_i)|\omega_l(\boldsymbol{x}_i), \text{data}_-, \mathbf{\Theta}_-\\&\sim \mathcal{N}\Bigg\{\text{ReLU}\{\omega_l(\boldsymbol{x})\} f_l(x) + \sum_{l'\neq l} \rho_{l'}(\boldsymbol{x}) f_{l'}(\boldsymbol{x})\\&\qquad + \boldsymbol{k}_\delta^T(\mathcal{X}_T^{[-i]}, \boldsymbol{x}_i)\boldsymbol{K}_\delta(\mathcal{X}_T^{[-i]}, \mathcal{X}_T^{[-i]})^{-1}\left(\boldsymbol{f}_{[-i],T} - \sum_l \boldsymbol{\rho}_l^{[-i]} \odot \boldsymbol{f}_l^{[-i]}\right),\\&\qquad k_\delta(\boldsymbol{x}_i, \boldsymbol{x}_i) - \boldsymbol{k}_\delta^T(\mathcal{X}_T^{[-i]}, \boldsymbol{x}_i)\boldsymbol{K}_\delta(\mathcal{X}_T^{[-i]}, \mathcal{X}_T^{[-i]})^{-1}\boldsymbol{k}_\delta(\mathcal{X}_T^{[-i]}, \boldsymbol{x}_i)\Bigg\}.\end{aligned} \tag{SM2.2}$$

The second term in (SM2.1) follows the standard GP for $\omega_l(\boldsymbol{x})$ conditional on $\boldsymbol{\omega}_l(\mathcal{X}_T^{[-i]})$:

$$\begin{aligned}&\omega_l(\boldsymbol{x}_i)|\text{data}_-, \mathbf{\Theta}_-\\&\sim \mathcal{N}\Big\{\boldsymbol{k}_{\omega_l}^T(\mathcal{X}_T^{[-i]}, \boldsymbol{x}_i)\boldsymbol{K}_{\omega_l}(\mathcal{X}_T^{[-i]}, \mathcal{X}_T^{[-i]})^{-1}\boldsymbol{\omega}_{[-i],l},\\&\qquad k_{\omega_l}(\boldsymbol{x}_i, \boldsymbol{x}_i) - \boldsymbol{k}_{\omega_l}^T(\mathcal{X}_T^{[-i]}, \boldsymbol{x}_i)\boldsymbol{K}_{\omega_l}(\mathcal{X}_T^{[-i]}, \mathcal{X}_T^{[-i]})^{-1}\boldsymbol{k}_{\omega_l}(\mathcal{X}_T^{[-i]}, \boldsymbol{x}_i)\Big\}\\&:= \mathcal{N}\{\mu_{i,l,-}, \sigma_{i,l,-}^2\}.\end{aligned} \tag{SM2.3}$$

Therefore, with Equations (SM2.1), (SM2.2), and (SM2.3), we can get that:

$$[\omega_l(\boldsymbol{x}_i)|\mathbf{\Theta}_-, \text{data}] = \begin{cases}\phi(\mu_{i,l,+}, \sigma_{i,l,+}^2), & \text{if } \omega_l(\boldsymbol{x}) > 0,\\ \phi(\mu_{i,l,-}, \sigma_{i,l,-}^2), & \text{if } \omega_l(\boldsymbol{x}) \leq 0,\end{cases}$$

where $\phi(\mu, \sigma^2)$ is the probability density function (PDF) of the normal distribution with mean $\mu$ and variance $\sigma^2$. For the first line, conditional on $\omega_l(\boldsymbol{x}) > 0$, $\mu_{i,l,+}$ and $\sigma_{i,l,+}^2$ (defined in (3.4) in the manuscript) can be calculated through multiplying the two PDFs in (SM2.2) and (SM2.3). For the second line, conditional on $\omega_l(\boldsymbol{x}) \leq 0$, the first term in (SM2.1) is a constant value independent on $\omega_l(\boldsymbol{x})$, thus the full conditional distribution equals to the second term. Define $\pi_{i,l}$ as the probability of $\omega_l(\boldsymbol{x}) > 0$. The ratio $\frac{\pi}{1-\pi}$ can be expressed as:

$$\frac{\pi_{i,l}}{1-\pi_{i,l}} = \frac{\int_0^\infty \phi(\mu_{i,l,+}, \sigma_{i,l,+}^2)}{\int_{-\infty}^0 \phi(\mu_{i,l,-}, \sigma_{i,l,-}^2)} = \Phi\left(\frac{\mu_{i,l,+}}{\sigma_{i,l,+}}\right) / \Phi\left(-\frac{\mu_{i,l,-}}{\sigma_{i,l,-}}\right). \tag{SM2.4}$$

Therefore, the full conditional distribution on $\omega_l(\boldsymbol{x})$ follows Equation (3.2) in the manuscript.

**SM3. Sampling details for the multi-fidelity LOL-GP.** For the multi-fidelity set-up, the set of latent parameters $\mathbf{\Theta}$ are defined as $\mathbf{\Theta} = \{\mathbf{\Theta}_1, \cdots, \mathbf{\Theta}_L\}$, where $\mathbf{\Theta}_l = \{\boldsymbol{\omega}_l(\mathcal{X}_{(l+1)}), \boldsymbol{f}_l(\mathcal{X}_{(l+1)})\}$. Here, for notational brevity, we presume that no design points are shared between any systems; Supplementary Materials SM provides analogous expressions for the setting with potentially shared design points.

For the $l$-th fidelity level, given data $= \{\boldsymbol{f}_1, \cdots, \boldsymbol{f}_{L+1}\}$, we can derive the following full conditional distributions for the latent weight parameters in $\mathbf{\Theta}_l$:

(SM3.1)
$$[\omega_l(\boldsymbol{x}_i)|\mathbf{\Theta}_{-}, \text{data}] \sim \pi_{i,l}\, \mathcal{N}_{\mathbb{R}^+}\{\mu_{i,l,+}, \sigma^2_{i,l,+}\} + (1-\pi_{i,l})\, \mathcal{N}_{\mathbb{R}^-}\{\mu_{i,l,-}, \sigma^2_{i,l,-}\}, \quad \boldsymbol{x}_i \in \mathcal{X}_{(l+1)}.$$

Here, the full conditional weights $\{\pi_{i,l}\}_{i,l}$ have the same form as equation (3.3) in the manuscript, with its means and variances given by:

(SM3.2)
$$\begin{aligned}
\mu_{i,l,-} &= \boldsymbol{k}^T_{\omega_l}(\mathcal{X}^{[-i]}_{(l+1)}, \boldsymbol{x}_i)\boldsymbol{K}_{\omega_l}(\mathcal{X}^{[-i]}_{(l+1)}, \mathcal{X}^{[-i]}_{(l+1)})^{-1}\boldsymbol{\omega}^{[-i]}_l,\\
\sigma^2_{i,l,-} &= k_{\omega_l}(\boldsymbol{x}_i, \boldsymbol{x}_i) - \boldsymbol{k}^T_{\omega_l}(\mathcal{X}^{[-i]}_{(l+1)}, \boldsymbol{x}_i)\boldsymbol{K}_{\omega_l}(\mathcal{X}^{[-i]}_{(l+1)}, \mathcal{X}^{[-i]}_{(l+1)})^{-1}\boldsymbol{k}_{\omega_l}(\mathcal{X}^{[-i]}_{(l+1)}, \boldsymbol{x}_i),\\
\mu_{i,l,+} &= \sigma^2_{i,l,+}\left(\frac{\mu_{i,l,-}}{\sigma^2_{i,l,-}} + \frac{f_{l+1}(\boldsymbol{x}_i) - \boldsymbol{k}^T_{\delta_l}(\mathcal{X}^{[-i]}_{(l+1)}, \boldsymbol{x}_i)\boldsymbol{K}_{\delta_l}(\mathcal{X}^{[-i]}_{(l+1)}, \mathcal{X}^{[-i]}_{(l+1)})^{-1}\left(\boldsymbol{f}^{[-i]}_{l+1} - \boldsymbol{\rho}^{[-i]}_l \odot \boldsymbol{f}^{[-i]}_l\right)}{\left[k_{\delta_l}(\boldsymbol{x}_i, \boldsymbol{x}_i) - \boldsymbol{k}^T_{\delta_l}(\mathcal{X}^{[-i]}_{(l+1)}, \boldsymbol{x}_i)\boldsymbol{K}_{\delta_l}(\mathcal{X}^{[-i]}_{(l+1)}, \mathcal{X}^{[-i]}_{(l+1)})^{-1}\boldsymbol{k}_{\delta_l}(\mathcal{X}^{[-i]}_{(l+1)}, \boldsymbol{x}_i)\right]/f_l(\boldsymbol{x}_i)}\right),\\
\sigma^2_{i,l,+} &= \left(\frac{1}{\sigma^2_{i,l,-}} + \frac{[f_l(\boldsymbol{x}_i)]^2}{k_{\delta_l}(\boldsymbol{x}_i, \boldsymbol{x}_l) - \boldsymbol{k}^T_{\delta_l}(\mathcal{X}^{[-i]}_{(l+1)}, \boldsymbol{x}_i)\boldsymbol{K}_{\delta_l}(\mathcal{X}^{[-i]}_{(l+1)}, \mathcal{X}^{[-i]}_{(l+1)})^{-1}\boldsymbol{k}_{\delta_l}(\mathcal{X}^{[-i]}_{(l+1)}, \boldsymbol{x}_i)}\right)^{-1}.
\end{aligned}$$

Here, $\mathcal{X}^{[-i]}_{(l+1)}$ denotes the set of $\mathcal{X}_{(l+1)}$ without the $i$-th point, and $\boldsymbol{\omega}^{[-i]}_l$, $\boldsymbol{\rho}^{[-i]}_l$, and $\boldsymbol{f}^{[-i]}_l$ are as defined in Section 3.2.

Similarly, we can derive the following full conditional distributions on the latent function values in $\mathbf{\Theta}_l$:

$$[f_l(\boldsymbol{x}_i)|\mathbf{\Theta}_{-}, \text{data}] \sim \mathcal{N}\{\mu_{i,l}, \sigma^2_{i,l}\}, \quad \boldsymbol{x}_i \in \mathcal{X}_{(l+1)}. \tag{SM3.3}$$

Here, the posterior means $\{\mu_{i,l}\}_{i,l}$ and variances $\{\sigma^2_{i,l}\}_{i,l}$ take the closed form expressions:

$$\mu_{i,l} = \boldsymbol{c}^T_l(\boldsymbol{x}_i)\boldsymbol{C}(\mathcal{X}^{[-i]}_{\text{aug}})^{-1}\boldsymbol{f}^{[-i]}_{\text{aug}}, \qquad \sigma^2_{i,l} = c_{l,l}(\boldsymbol{x}_i, \boldsymbol{x}_i) - \boldsymbol{c}^T_l(\boldsymbol{x}_i)\boldsymbol{C}(\mathcal{X}^{[-i]}_{\text{aug}})^{-1}\boldsymbol{c}_l(\boldsymbol{x}_i), \tag{SM3.4}$$

where $\boldsymbol{f}_{\text{aug}} = [\boldsymbol{f}_l(\mathcal{X}_{(l)})]^{L+1}_{l=1}$ and $\boldsymbol{f}^{[-i]}_{\text{aug}}$ omits its $i$-th point. In this expression, $c_{l,l}(\boldsymbol{x}_i, \boldsymbol{x}_i)$ is the prior variance of $f_l(\boldsymbol{x}_i)$, $\boldsymbol{c}_l(\boldsymbol{x}_i)$ is the prior covariance vector between $f_l(\boldsymbol{x}_i)$ and $\boldsymbol{f}^{[-i]}_{\text{aug}}$, and $\boldsymbol{C}(\mathcal{X}^{[-i]}_{\text{aug}})$ is the prior covariance matrix for $\boldsymbol{f}^{[-i]}_{\text{aug}}$. Such covariances can be directly computed using the modeling equations in (3.9) of the main paper:

$$\begin{aligned}
&\text{cov}_{1,1}(\boldsymbol{x}, \boldsymbol{x}') = k(\boldsymbol{x}, \boldsymbol{x}')\\
&\text{cov}_{l,l}(\boldsymbol{x}, \boldsymbol{x}') = \rho_l(\boldsymbol{x})\rho_l(\boldsymbol{x}')\text{cov}_{l-1,l-1}(\boldsymbol{x}, \boldsymbol{x}') + k_{\delta_{l-1}}(\boldsymbol{x}, \boldsymbol{x}'),\ 2 \leq l \leq L+1\\
&\text{cov}_{l,l'}(\boldsymbol{x}, \boldsymbol{x}') = \left[\prod_{j=l'}^{l-1} \rho_j(\boldsymbol{x}')\right] \text{cov}_{j,j}(\boldsymbol{x}, \boldsymbol{x}'),\ 1 \leq l' < l \leq L+1.
\end{aligned} \tag{SM3.5}$$

The key appeal is that the above closed-form full conditionals (SM3.2) and (SM3.4) permit *efficient* Gibbs sampling of the posterior distribution $[\boldsymbol{\Theta}|\text{data}]$; see Algorithm SM3.1.

The following equation (Eq (3.12) in the main text) provides the roadmap for efficient posterior sampling from the desired predictive distribution $[f_{L+1}(\boldsymbol{x}_{\text{new}})|\text{data}]$:

$$[f_{L+1}(\boldsymbol{x}_{\text{new}})|\text{data}] = \int \text{Ⓐ}_{L+1} \cdots \text{Ⓐ}_1 \text{Ⓑ} \, df_L(\boldsymbol{x}_{\text{new}}) \cdots df_1(\boldsymbol{x}_{\text{new}}) \, d\boldsymbol{\Theta},$$

Note that distribution Ⓑ has already sampled via our earlier Gibbs sampler using (SM3.1) and (SM3.3). The distribution $\text{Ⓐ}_1$ follows the standard GP posterior distribution on $f_1(\cdot)$, conditioned on data $\boldsymbol{f}_1(\mathcal{X}_1)$ and latent observations $\boldsymbol{f}_1(\mathcal{X}_{(2)})$ from $\boldsymbol{\Theta}$. Each of the distributions in $\{\text{Ⓐ}_{l+1}\}_{l=1}^{L}$ can then be sampled via Monte Carlo in two steps. First (i), draw a sample from $[\omega_l(\boldsymbol{x}_{\text{new}})|\boldsymbol{\Theta}, \text{data}]$, which follows an independent normal distribution from the standard GP equations (2.3) for $\omega_l(\cdot)$ conditional on $\omega_l(\mathcal{X}_{(l+1)})$. Next (ii), with $f_l(\boldsymbol{x}_{\text{new}})$ and $\omega_l(\boldsymbol{x}_{\text{new}})$ in hand, sample $f_{l+1}(\boldsymbol{x}_{\text{new}})$ from:

$$\begin{aligned}
&[f_{l+1}(\boldsymbol{x}_{\text{new}})|f_l(\boldsymbol{x}_{\text{new}}), \omega_l(\boldsymbol{x}_{\text{new}}), \boldsymbol{\Theta}, \text{data}] \\
&\quad \sim \mathcal{N}\Big\{\rho_l(\boldsymbol{x}_{\text{new}})f_l(\boldsymbol{x}_{\text{new}}) + \boldsymbol{k}_{\delta_l}^T(\mathcal{X}_{(l+1)}, \boldsymbol{x}_{\text{new}})\boldsymbol{K}_{\delta_l}(\mathcal{X}_{(l+1)}, \mathcal{X}_{(l+1)})^{-1} \\
&\qquad\qquad \cdot \left[\boldsymbol{f}_{l+1}(\mathcal{X}_{(l+1)}) - \boldsymbol{\rho}_l(\mathcal{X}_{(l+1)}) \odot \boldsymbol{f}_l(\mathcal{X}_{(l+1)})\right], \\
&\qquad k_{\delta_l}(\boldsymbol{x}_{\text{new}}, \boldsymbol{x}_{\text{new}}) - \boldsymbol{k}_{\delta_l}^T(\mathcal{X}_{(l+1)}, \boldsymbol{x}_{\text{new}})\boldsymbol{K}_{\delta_l}(\mathcal{X}_{(l+1)}, \mathcal{X}_{(l+1)})^{-1}\boldsymbol{k}_{\delta_l}(\mathcal{X}_{(l+1)}, \boldsymbol{x}_{\text{new}})\Big\}.
\end{aligned} \tag{SM3.6}$$

With this, we can finally construct the posterior sampler for $[f_{L+1}(\boldsymbol{x}_{\text{new}})|\text{data}]$. First, take a sample $\boldsymbol{\Theta}_{[b]}$ from the MCMC chain for $[\boldsymbol{\Theta}|\text{data}]$. Next, with $\boldsymbol{\Theta} = \boldsymbol{\Theta}_{[b]}$, sample $f_1(\boldsymbol{x}_{\text{new}})$ from $\text{Ⓐ}_1$, sample $f_2(\boldsymbol{x}_{\text{new}})$ from $\text{Ⓐ}_2$, and so until $f_{L+1}(\boldsymbol{x}_{\text{new}})$ is sampled from $\text{Ⓐ}_{L+1}$. The resulting sample follows the desired posterior distribution $[f_{L+1}(\boldsymbol{x}_{\text{new}})|\text{data}]$ from (3.12). One can then repeat this procedure for all samples in the MCMC chain $\{\boldsymbol{\Theta}_{[b]}\}_{b=1}^{B}$ to obtain corresponding MCMC samples for the high-fidelity output $f_{L+1}(\boldsymbol{x}_{\text{new}})$. Algorithm SM3.1 summarizes this posterior predictive sampler for the multi-fidelity LOL-GP.

**SM4. Full expressions for Equation (4.1).** Recall that Equation (4.1) in the main paper provides the optimization formulation for approximate MAP estimation, namely:

$$\hat{\boldsymbol{\Xi}} = \arg\max_{\boldsymbol{\Xi}} \log\left\{[\text{data}|\hat{\boldsymbol{\Theta}}, \boldsymbol{\Xi}]\ [\hat{\boldsymbol{\Theta}}|\boldsymbol{\Xi}]\ [\boldsymbol{\Xi}]\right\}. \tag{SM4.1}$$

Consider first the multi-source LOL-GP. Note that the data follows the following joint distribution:

$$\begin{pmatrix} \boldsymbol{f}_1 \\ \vdots \\ \boldsymbol{f}_L \\ \boldsymbol{f}_T \end{pmatrix} |\boldsymbol{\Xi}, \hat{\boldsymbol{\Theta}} \sim \mathcal{N}\left(\begin{bmatrix} \boldsymbol{0} \\ \vdots \\ \boldsymbol{0} \\ \boldsymbol{0} \end{bmatrix}, \left[\begin{array}{ccc|c} \boldsymbol{K}_{1,1} & \cdots & \boldsymbol{0} & \boldsymbol{K}_{1,T} \\ \vdots & \ddots & \vdots & \vdots \\ \boldsymbol{0} & \cdots & \boldsymbol{K}_{L,L} & \boldsymbol{K}_{L,T} \\ \hline \boldsymbol{K}_{1,L}^T & \cdots & \boldsymbol{K}_{L,T}^T & \boldsymbol{K}_{T,T} \end{array}\right]\right) =: \mathcal{N}\left(\boldsymbol{0}, \boldsymbol{K}_f\right). \tag{SM4.2}$$

Here, $\boldsymbol{K}_{l,l'} = \text{cov}_{l,l'}(\mathcal{X}_l, \mathcal{X}_{l'})$ is the cross-covariance matrix between $\boldsymbol{f}_l$ and $\boldsymbol{f}_{l'}$, which can easily

**Algorithm SM3.1** Multi-fidelity LOL-GP: Gibbs sampling and posterior predictive sampling

*Require*: Multi-fidelity data $\{(\mathcal{X}_l, \boldsymbol{f}_l)\}_{l=1}^{L+1}$, number of MCMC iterations $B$, initial MCMC parameters $\boldsymbol{\Theta}_{[0]}$.

*Gibbs Sampling of* $[\boldsymbol{\Theta}|\text{data}]$:

- Initialize $\boldsymbol{\Theta} \leftarrow \boldsymbol{\Theta}_{[0]}$ in the MCMC chain.

**for** $b = 1, \cdots, B$ **do**
  - Set $\boldsymbol{\Theta} \leftarrow \boldsymbol{\Theta}_{[b-1]}$.

  **for** $l = 1, \cdots, L$ **do**
    **for** $i = 1, \cdots, \sum_{l'=l+1}^{L+1} n_{l'}$ **do**
      - For $\boldsymbol{x}_i \in \mathcal{X}_{(l+1)}$, update $\omega_l(\boldsymbol{x}_i)$ in $\boldsymbol{\Theta}_l$ by sampling from the full conditional distribution (SM3.1).
      - For $\boldsymbol{x}_i \in \mathcal{X}_{(l+1)}$, update $f_l(\boldsymbol{x}_i)$ in $\boldsymbol{\Theta}_l$ by sampling from the full conditional distribution (SM3.3).

    **end for**
  **end for**
  - Update $\boldsymbol{\Theta}_{[b]} \leftarrow \boldsymbol{\Theta}$.

**end for**

*Return*: MCMC samples $\{\boldsymbol{\Theta}_{[b]}\}_{b=1}^{B}$.

*Posterior Predictive Sampling of* $[f_{L+1}(\boldsymbol{x}_{\text{new}})|\text{data}]$:

- Denote $\{\omega_{l,[b]}\}_{b=1}^{B}$ and $\{f_{l,[b]}\}_{b=1}^{B}$ as the posterior samples for $\omega_l(\boldsymbol{x}_{\text{new}})$ and $f_l(\boldsymbol{x}_{\text{new}})$.

**for** $b = 1, \cdots, B$ **do**
  - Sample $$f_{1,[b]} \sim \mathcal{N}\big\{\boldsymbol{k}_1^T(\mathcal{X}_{(1)}, \boldsymbol{x}_{\text{new}})\boldsymbol{K}_1(\mathcal{X}_{(1)}, \mathcal{X}_{(1)})^{-1}\boldsymbol{f}_1(\mathcal{X}_{(1)}),\; k_1(\boldsymbol{x}_{\text{new}}, \boldsymbol{x}_{\text{new}}) - \boldsymbol{k}_1^T(\mathcal{X}_{(1)}, \boldsymbol{x}_{\text{new}})\boldsymbol{K}_1(\mathcal{X}_{(1)}, \mathcal{X}_{(1)})^{-1}\boldsymbol{k}_1(\mathcal{X}_{(1)}, \boldsymbol{x}_{\text{new}})\big\}.$$
  with $f_1(\mathcal{X}_{(1)})$ from $\boldsymbol{\Theta}_{[b]}$.

**end for**

**for** $l = 1, \cdots, L$ **do**
  **for** $b = 1, \cdots, B$ **do**
    - Sample $$\omega_{l,[b]} \sim \mathcal{N}\big\{\boldsymbol{k}_{\omega_l}^T(\mathcal{X}_{(l+1)}, \boldsymbol{x}_{\text{new}})\boldsymbol{K}_{\omega_l}^{-1}(\mathcal{X}_{(l+1)}, \mathcal{X}_{(l+1)})\boldsymbol{\omega}_l(\mathcal{X}_{(l+1)}),\; k_{\omega_l}(\boldsymbol{x}_{\text{new}}, \boldsymbol{x}_{\text{new}}) - \boldsymbol{k}_{\omega_l}^T(\mathcal{X}_{(l+1)}, \boldsymbol{x}_{\text{new}})\boldsymbol{K}_{\omega_l}^{-1}(\mathcal{X}_{(l+1)}, \mathcal{X}_{(l+1)})\boldsymbol{k}_{\omega_l}(\mathcal{X}_{(l+1)}, \boldsymbol{x}_{\text{new}})\big\}.$$
    with $\omega_l(\mathcal{X}_{(l)})$ from $\boldsymbol{\Theta}_{[b]}$.
    - Sample $f_{l+1,[b]}$ from the full conditional distribution (SM3.6) with $f_{l,[b]}$ and $\omega_{l,[b]}$.

  **end for**
**end for**

*Return*: MCMC samples $\{f_{L+1,[b]}\}_{b=1}^{B}$ on $f_{L+1}(\boldsymbol{x}_{\text{new}})$.

be derived from the modeling equations in (3.1) of the main paper. From this, we thus have:

$$\text{(SM4.3)} \qquad \left[\text{data}|\boldsymbol{\Xi}, \hat{\boldsymbol{\Theta}}\right] = \prod_{l=1}^{L} \phi(\boldsymbol{f}_l|\boldsymbol{0}, \boldsymbol{K}_{l,l})\phi(\boldsymbol{f}_T|\tilde{\boldsymbol{z}}_T, \boldsymbol{H}_T),$$

where $\phi(\cdot|\boldsymbol{\mu}, \boldsymbol{\Sigma})$ is the multivariate normal density. The marginal mean vector and covariance

matrix for $\boldsymbol{f}_T$ is then given by:

$$\tilde{\boldsymbol{z}}_T = \sum_{l=1}^{L} [(\mathbf{1}_{n_l}\boldsymbol{\rho}_l^T(\mathcal{X}_T)) \odot \boldsymbol{K}_l(\mathcal{X}_l,\mathcal{X}_T)]^T \boldsymbol{K}_l^{-1}(\mathcal{X}_l,\mathcal{X}_l)\boldsymbol{f}_l,$$

$$\boldsymbol{H}_T = \boldsymbol{K}_\delta(\mathcal{X}_T,\mathcal{X}_T) + \sum_{l=1}^{L}[\boldsymbol{\rho}_l(\mathcal{X}_T)\boldsymbol{\rho}_l^T(\mathcal{X}_T)] \odot \boldsymbol{K}_l(\mathcal{X}_T,\mathcal{X}_T) - \sum_{l=1}^{L} \left[(\mathbf{1}_{n_l}\boldsymbol{\rho}_l^T(\mathcal{X}_T)) \odot \boldsymbol{K}_l(\mathcal{X}_l,\mathcal{X}_T)\right]^T \boldsymbol{K}_l^{-1}(\mathcal{X}_l,\mathcal{X}_l) \left[(\mathbf{1}_{n_l}\boldsymbol{\rho}_l^T(\mathcal{X}_T)) \odot \boldsymbol{K}_l(\mathcal{X}_l,\mathcal{X}_T)\right].$$

Finally, $[\hat{\boldsymbol{\Theta}}|\boldsymbol{\Xi}]$ follows immediately from the marginal GP equations for $\hat{\boldsymbol{\Theta}}$.

Consider next the multi-fidelity LOL-GP. Here, one can show that:

$$[\text{data}|\boldsymbol{\Xi},\hat{\boldsymbol{\Theta}}] \propto \frac{1}{|\boldsymbol{C}_{1:(L+1)}|} \exp\left\{-\frac{1}{2}\boldsymbol{f}_{1:(L+1)}^T \boldsymbol{C}_{1:(L+1)}^{-1} \boldsymbol{f}_{1:(L+1)}\right\}, \tag{SM4.4}$$

where $\boldsymbol{C}_{1:(L+1)}$ is the covariance matrix defined in Equation (4.4) of the main paper. As before, $[\hat{\boldsymbol{\Theta}}|\boldsymbol{\Xi}]$ follows immediately from the marginal GP equations for $\hat{\boldsymbol{\Theta}}$.

**SM5. Nested design for the multi-source LOL-GP.** We consider here a recursive formulation of the multi-source LOL-GP given the design points possess a nested property, i.e., $\mathcal{X}_T \subset \mathcal{X}_l$, for all $l = 1, \cdots, L$. With such a nested design, the multi-source LOL-GP can be formulated recursively as:

$$\begin{aligned} f_T(\boldsymbol{x}) &= \sum_{l=1}^{L} \rho_l(\boldsymbol{x})\tilde{f}_l(\boldsymbol{x}) + \delta(\boldsymbol{x}), \\ \tilde{f}_l(\boldsymbol{x}) &= [f_l(\boldsymbol{x})|\boldsymbol{f}_l] \sim \mathcal{N}(\tilde{\mu}_l(\boldsymbol{x}), \tilde{\sigma}_l^2(\boldsymbol{x})), \end{aligned} \tag{SM5.1}$$

Here, $\tilde{f}_l(\boldsymbol{x})$ is the GP conditional on data $\boldsymbol{f}_l$, with mean and variance:

$$\begin{aligned} \tilde{\mu}_l(\boldsymbol{x}) &= \boldsymbol{K}_l^T(\mathcal{X}_l,\boldsymbol{x})\boldsymbol{K}_l^{-1}(\mathcal{X}_l,\mathcal{X}_l)\boldsymbol{f}_l, \\ \tilde{\sigma}_l^2(\boldsymbol{x}) &= k_l(\boldsymbol{x},\boldsymbol{x}) - \boldsymbol{K}_l^T(\mathcal{X}_l,\boldsymbol{x})\boldsymbol{K}_l^{-1}(\mathcal{X}_l,\mathcal{X}_l)\boldsymbol{K}_l(\mathcal{X}_l,\boldsymbol{x}). \end{aligned}$$

Here, due to the nested design, we know the exact values of $f_l(\mathcal{X}_T)$ as this is a subset of $\boldsymbol{f}_l$. Such values thus do not need to be sampled within the Gibbs sampler, whereas other sampling steps remain the same. The complexity of the Gibbs sampler then reduces to $\mathcal{O}\left\{2Ln_T^2\right\}$ per iteration. For hyperparameter optimization, $\boldsymbol{z}_T$ and $\boldsymbol{H}_T$ can be simplified to:

$$\boldsymbol{z}_T = \boldsymbol{f}_T - \sum_{l=1}^{L} \rho_l(\mathcal{X}_T) \odot f_l(\mathcal{X}_T), \quad \boldsymbol{H}_T = \boldsymbol{K}_\delta(\mathcal{X}_T,\mathcal{X}_T).$$

Note that this does not change the per-evaluation cost of the objective for hyperparameter optimization.

**SM6. Modeling architecture and additional experiments for BTLNet.** We first provide details on the modeling architecture for BTLNet. For the multi-source experiments, the responses of source systems are modeled via a fully-connected neural network with linear layers. The Bayesian neural network for the target system uses the linear variational layers from [SM1], and takes the outputs of all source models and the target design point as input. ReLU activation functions are used within all networks. Table SM1 summarizes the network structures used in the multi-source experiments, which have been optimized via manual tuning.

| | Number of hidden layers | Size of hidden layers |
|---|---|---|
| Forrester | 1st source: 3<br>2nd source: 3<br>Target: 2 | 1st source: 20<br>2nd source: 20<br>Target: 10 |
| Friedman | 1st source: 3<br>2nd source: 3<br>Target: 1 | 1st source: 25<br>2nd source: 25<br>Target: 10 |
| Jet turbine | Source: 3<br>Target: 1 | Source: 20<br>Target: 15 |

Table SM1: Network structure of BTLNet for multi-source experiments.

For the multi-fidelity experiments, we take a fully-connected neural network with linear layers and ReLU activation functions for each fidelity level, and its output is fed as inputs (along with corresponding design points) into the networks of higher-fidelity levels. Table SM2 summarizes the network structures used in the multi-fidelity experiments, which have been optimized via manual tuning.

| | Number of hidden layers | Size of hidden layers |
|---|---|---|
| Forrester | Low-fidelity: 2<br>High-fidelity: 1 | Low-fidelity: 16<br>High-fidelity: 64 |
| Branin | Low-fidelity: 2<br>Mid-fidelity: 2<br>High-fidelity: 1 | Low-fidelity: 12<br>Mid-fidelity: 8<br>High-fidelity: 8 |
| Jet turbine | Low-fidelity: 3<br>Mid-fidelity: 3<br>High-fidelity: 1 | Low-fidelity: 20<br>Mid-fidelity: 15<br>High-fidelity: 15 |

Table SM2: Network structure of BTLNet for multi-fidelity experiments.

Additionally, we investigated the performance of BTLNet with different choices of network structures and activation functions. For network structure, we employed an alternate deeper structure with more hidden layers and hidden units (details in Table SM4). For activation functions, we explored the use of sigmoid functions. Table SM3 summarizes the metrics

for the four resulting variants of BTLNet (two choices of network structures, two choices of activation functions). We can see that BTLNet yields the best performance using the selected network structure with ReLU activation functions. Here, a deeper network structure may not be beneficial due to the limited amount of target training data. The sigmoid function yields worse performance (particularly with a deeper network structure), perhaps due to the gradient vanishing phenomena [SM2].

| | Multi-source | | | | Multi-fidelity | | | |
|---|---|---|---|---|---|---|---|---|
| | Forrester | | Friedman | | Forrester | | Branin | |
| | RMSE | CRPS | RMSE | CRPS | RMSE | CRPS | RMSE | CRPS |
| **BTLNet-ReLU (Selected structure)** | **0.398** | **0.202** | **0.372** | **0.199** | **0.205** | **0.102** | **0.258** | **0.134** |
| BTLNet-Sigmoid (Selected structure) | 0.499 | 0.309 | 0.479 | 0.286 | 0.437 | 0.267 | 0.496 | 0.323 |
| BTLNet-ReLU (Deeper structure) | 0.411 | 0.205 | 0.377 | 0.200 | 0.252 | 0.122 | 0.283 | 0.149 |
| BTLNet-Sigmoid (Deeper structure) | 0.914 | 0.513 | 0.741 | 0.519 | 0.515 | 0.320 | 0.571 | 0.422 |

Table SM3: Predictive metrics for the four variants of BTLNet with different choices of architectures and activation functions for numerical experiments.

| | Number of hidden layers | Size of hidden layers |
|---|---|---|
| Multi-source Forrester | 1st source: 4<br>2nd source: 4<br>Target: 3 | 1st source: 30<br>2nd source: 30<br>Target: 15 |
| Multi-source Friedman | 1st source: 4<br>2nd source: 4<br>Target: 2 | 1st source: 36<br>2nd source: 36<br>Target: 15 |
| Multi-fidelity Forrester | Low-fidelity: 2<br>High-fidelity: 2 | Low-fidelity: 32<br>High-fidelity: 64 |
| Multi-fidelity Branin | Low-fidelity: 3<br>Mid-fidelity: 2<br>High-fidelity: 2 | Low-fidelity: 20<br>Mid-fidelity: 15<br>High-fidelity: 15 |

Table SM4: Deeper network structure of BTLNet for numerical experiments.

## REFERENCES


[1] X. Meng, H. Babaee, and G. E. Karniadakis, *Multi-fidelity Bayesian neural networks: Algorithms and applications*, Journal of Computational Physics, 438 (2021), p. 110361.

[2] A. Rehmer and A. Kroll, *On the vanishing and exploding gradient problem in gated recurrent units*, IFAC-PapersOnLine, 53 (2020), pp. 1243–1248.
